# Supplementary material for: The High W Challenge: Robust Neutrino Energy Estimators for LArTPCs
Source: arXiv:2511.11149 ancillary file (2026-06-02)
Supplement: Supplementary file 1 [file PRD_Neutrino_Energy_Estimator_SupMat.pdf]

# The High W Challenge: Robust Neutrino Energy Estimators for LArTPCs - Supplemental Material

November 14, 2025

## 1 Response

We include the response matrices for all generator and estimator combinations. The CCQE-like method is shown in Fig. 1, the $W^2$ method in Fig. 2, the proton based method in Fig. 3, the calorimetric technique in Fig. 4, and the Sobczyk-Furmanski method [2] in Fig. 5. Comparison of the features of each estimator across the four generators indicates the responses shown from the GENIE generator in the article are representative of the other three generators. We also compare the fraction error distributions, before and after applying detector resolution effects, in Figs. 6 and 7 respectively.

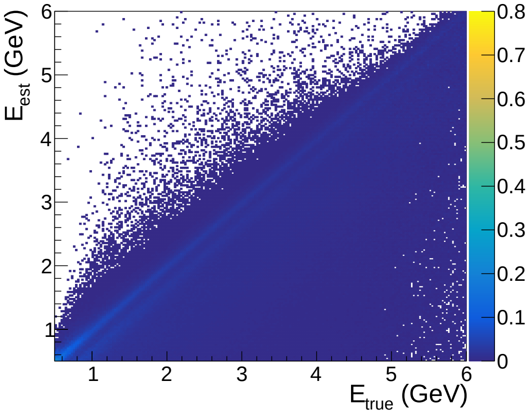


(a) GENIE.

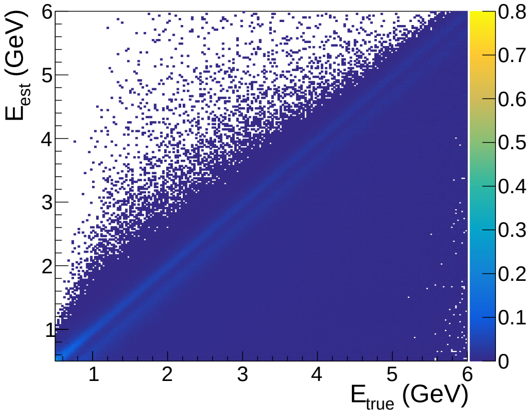


(b) NuWro.

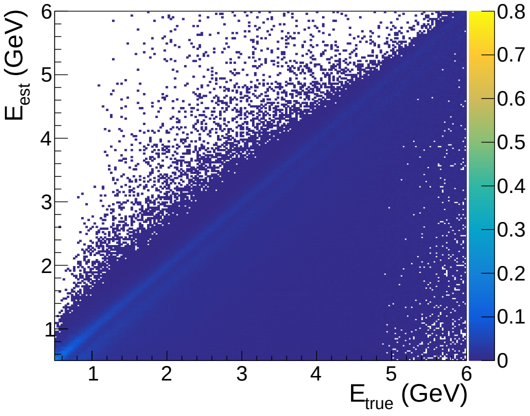


(c) NEUT.

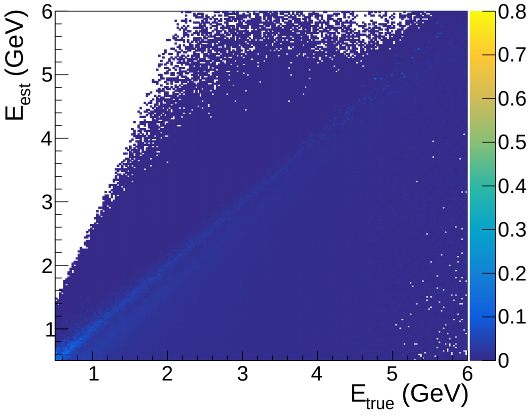


(d) GiBUU.

Figure 1: Response matrices describing the smearing from true neutrino energy to estimated neutrino energy using the CCQE-like method for each event generator.

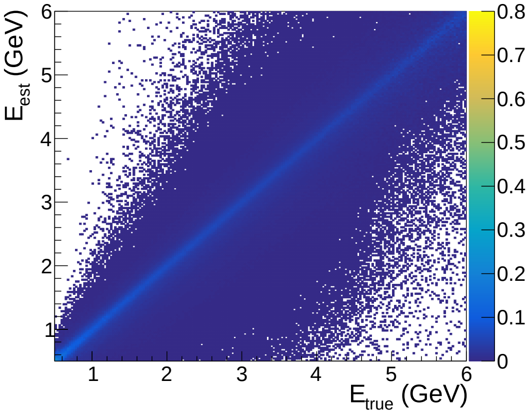


(a) GENIE.

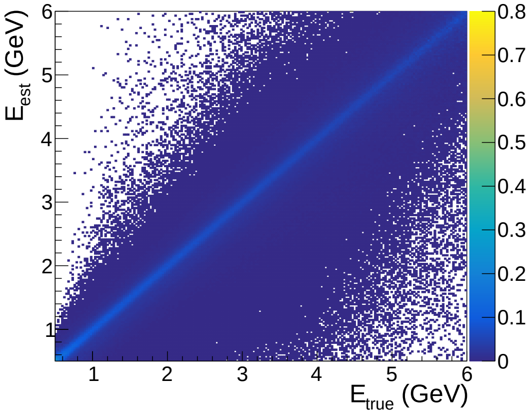


(b) NuWro.

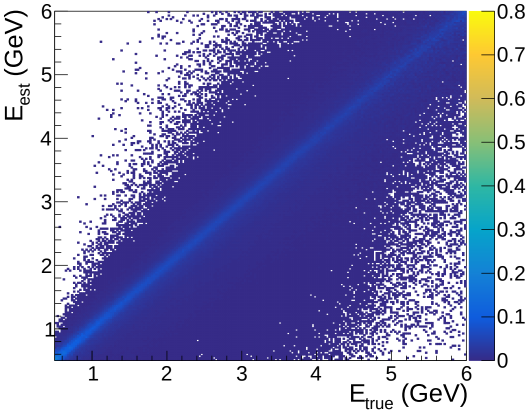


(c) NEUT.

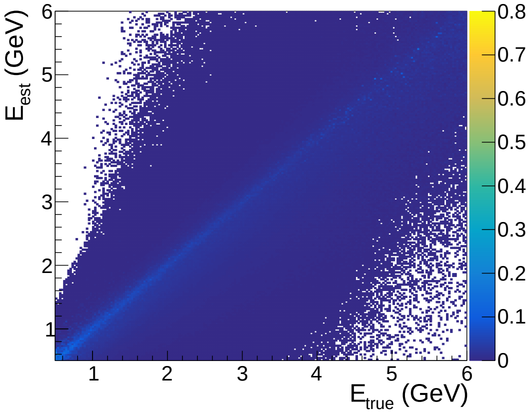


(d) GiBUU.

Figure 2: Response matrices describing the smearing from true neutrino energy to estimated neutrino energy using the $W^2$ method for each event generator.

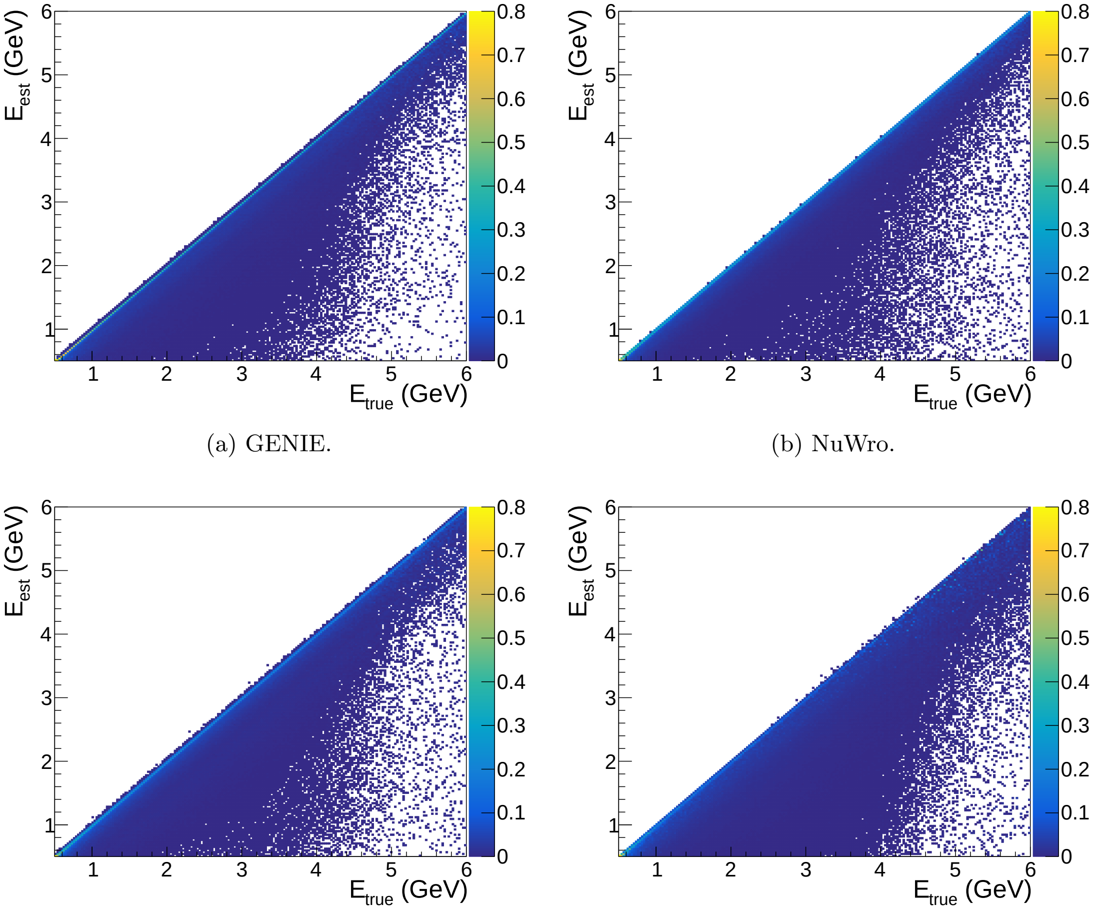


(a) GENIE.

(b) NuWro.

(c) NEUT.

(d) GiBUU.

Figure 3: Response matrices describing the smearing from true neutrino energy to estimated neutrino energy using the proton-based method for each event generator.

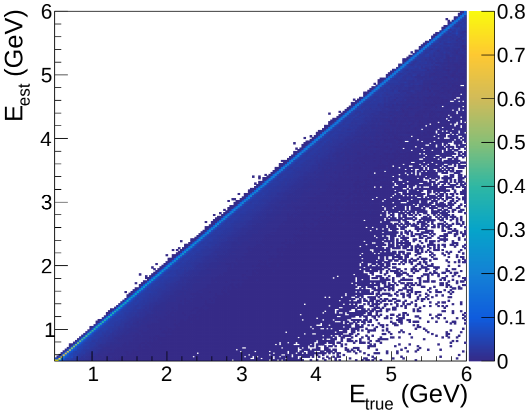


(a) GENIE.

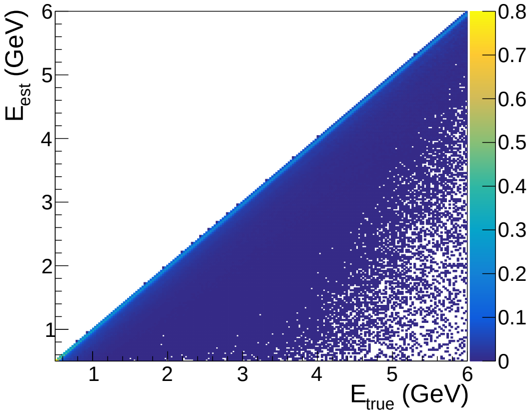


(b) NuWro.

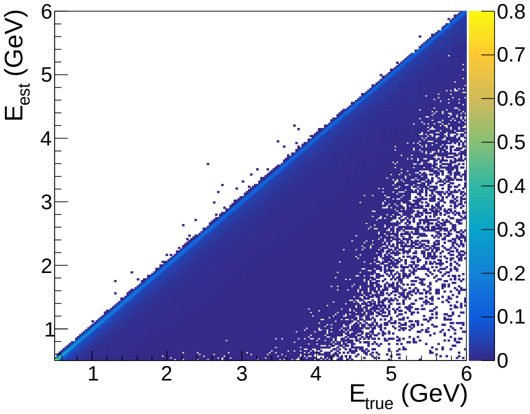


(c) NEUT.

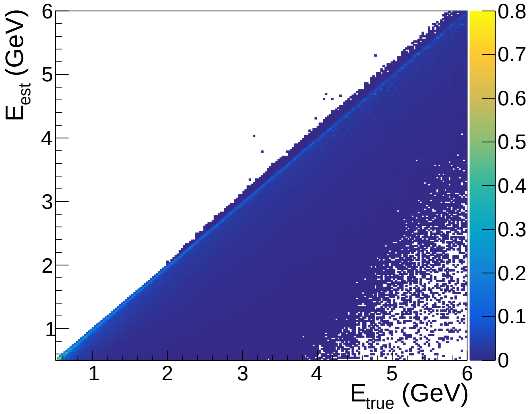


(d) GiBUU.

Figure 4: Response matrices describing the smearing from true neutrino energy to estimated neutrino energy using the calorimetric method for each event generator.

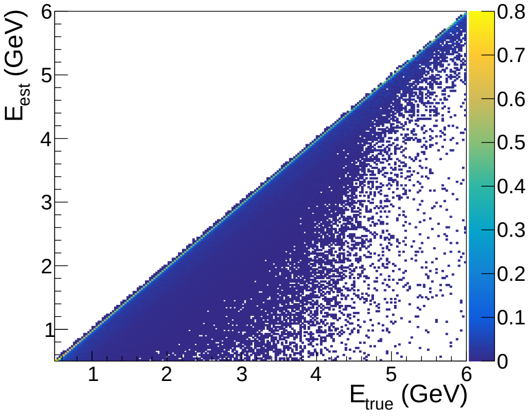


(a) GENIE.

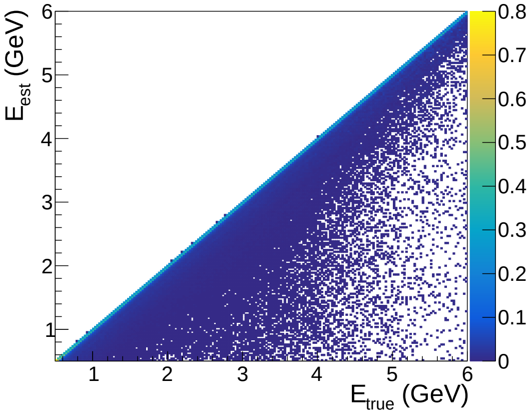


(b) NuWro.

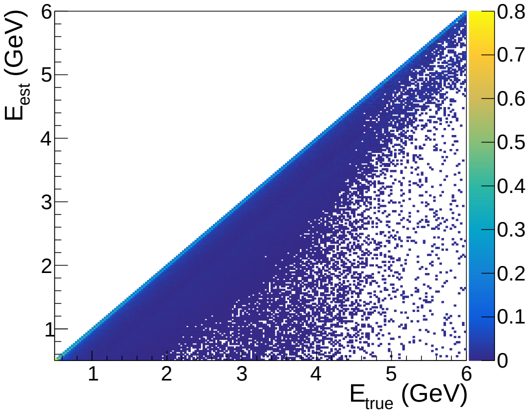


(c) NEUT.

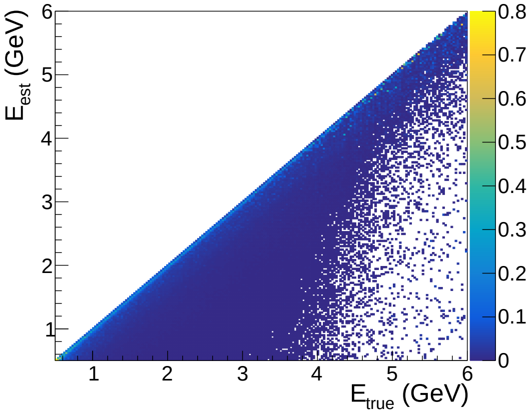


(d) GiBUU.

Figure 5: Response matrices describing the smearing from true neutrino energy to estimated neutrino energy using the Sobczyk-Furmanski method for each event generator.

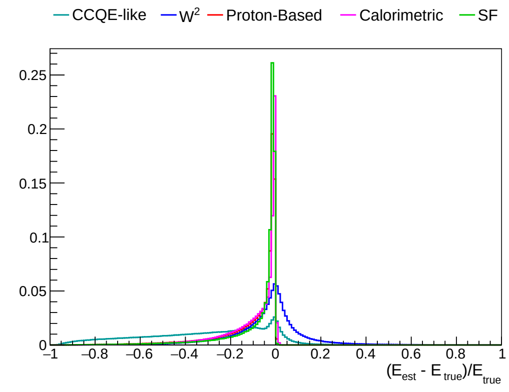


(a) GENIE.

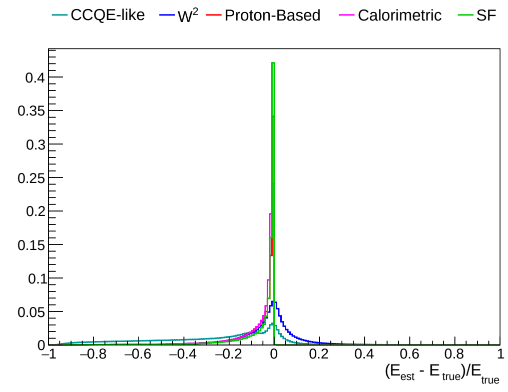


(b) NuWro.

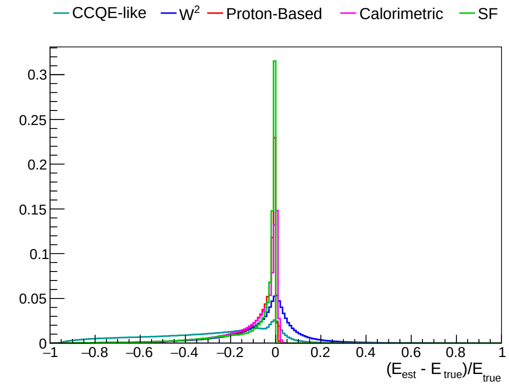


(c) NEUT.

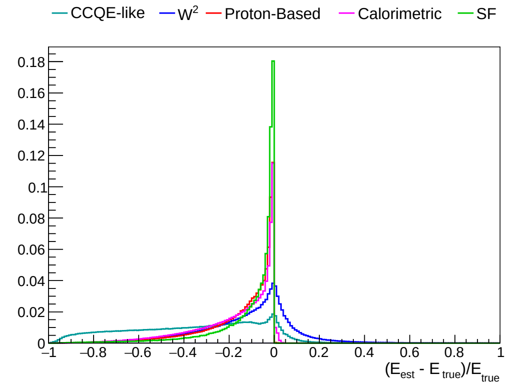


(d) GiBUU.

Figure 6: Distributions of fractional error in neutrino energy from each estimator calculated for the four neutrino event generators studied.

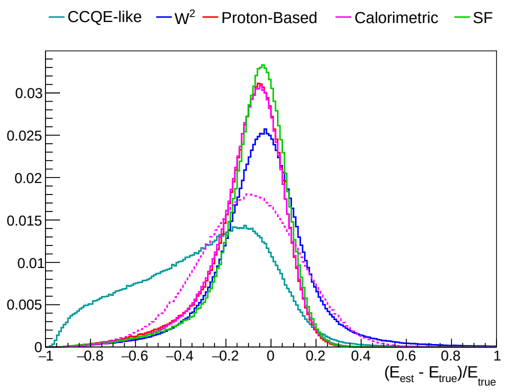


(a) GENIE.

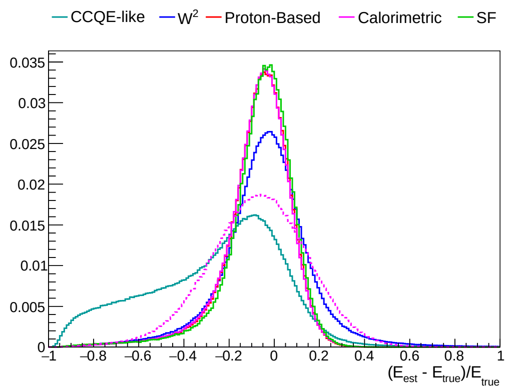


(b) NuWro.

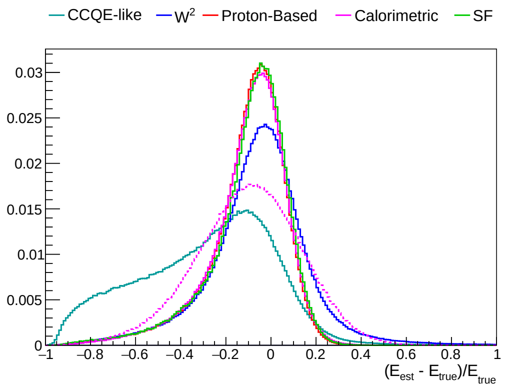


(c) NEUT.

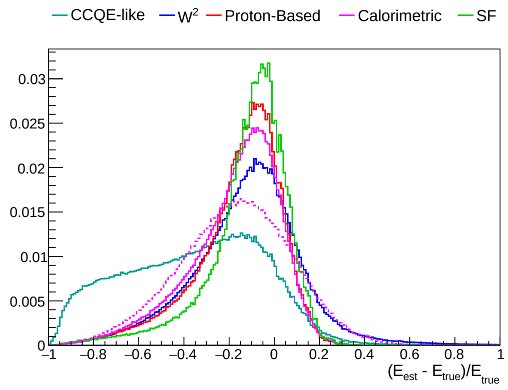


(d) GiBUU.

Figure 7: Distributions of fractional error in neutrino energy from each estimator calculated for the four neutrino event generators studied, after applying detector resolution effects. The dashed pink line indicates the performance of the calorimetric method when applying the overall 20% smearing to the estimated energy.

# 2 Variance with Different Generators

We present the variance in estimated neutrino energy resulting from each neutrino event generator.

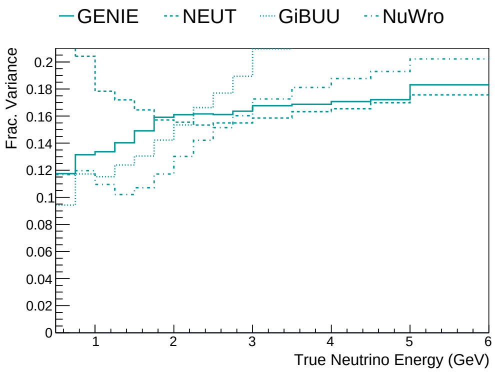


(a) CCQE-like method.

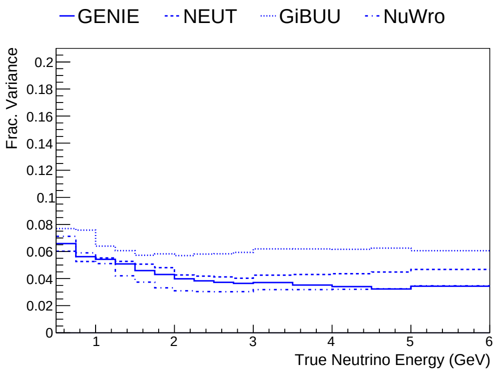


(b) $W^2$ method.

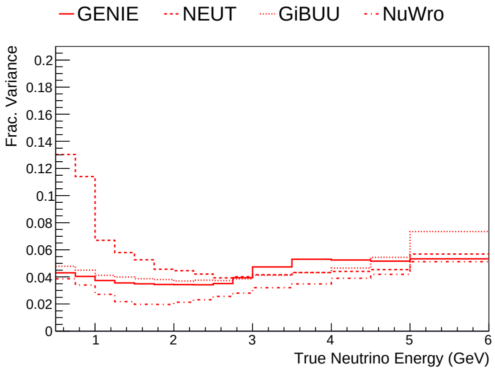


(c) Proton kinematics.

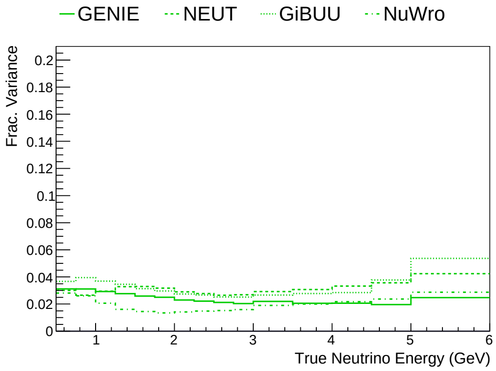


(d) SF method.

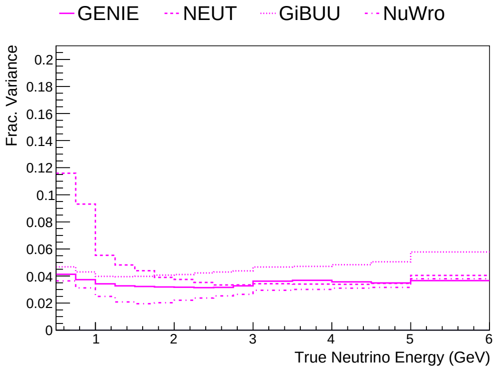


(e) Calorimetric method.

Figure 8: Variance in estimated neutrino energy as a function of true neutrino energy.

# 3 Bias as a Function of Secondary Variables

Below we show the bias distributions for each secondary variable for each generator, with the visible hadronic mass in Fig. 9, missing hadronic energy in Fig. 10, and lepton scattering angle in Fig. 11.

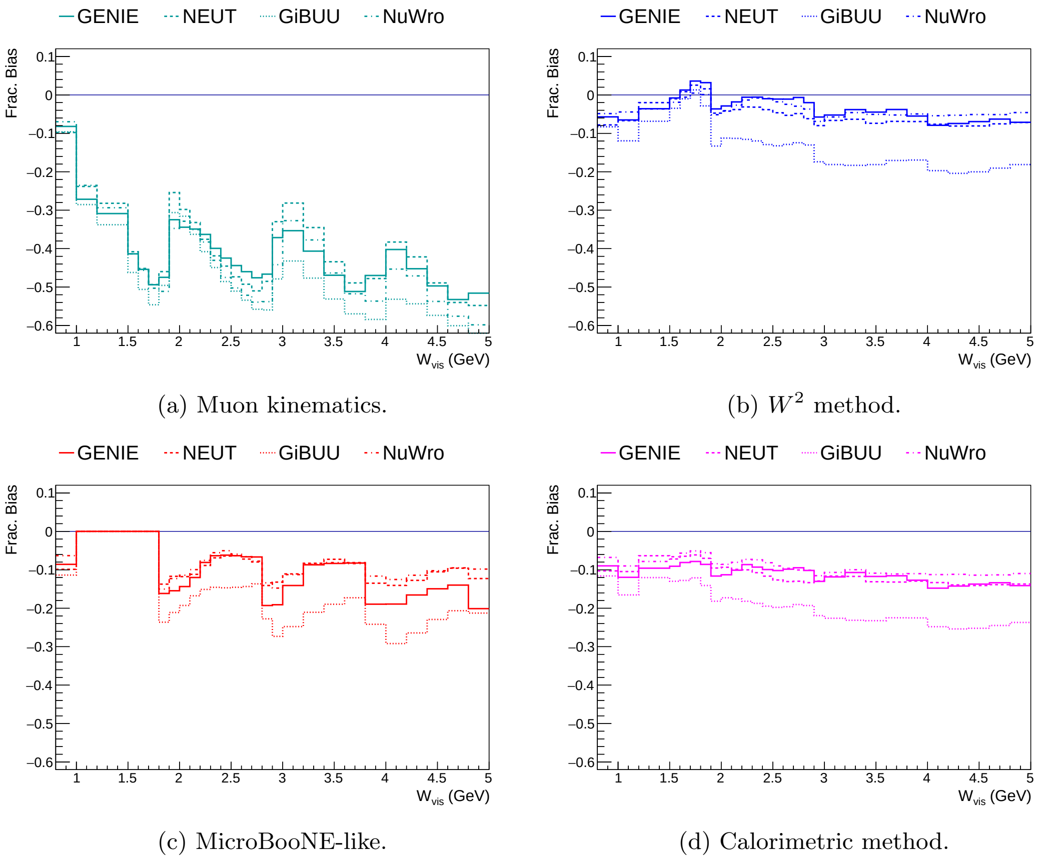


(a) Muon kinematics.

(b) $W^2$ method.

(c) MicroBooNE-like.

(d) Calorimetric method.

Figure 9: Testing the robustness of each neutrino energy estimation method with respect to different models by calculating the fractional bias as a function of visible hadronic invariant mass, and comparing the results from different event generators.

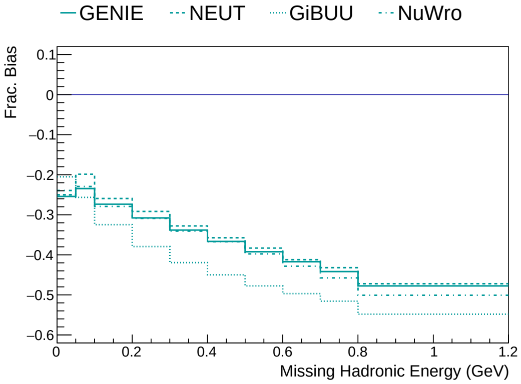


(a) Muon kinematics.

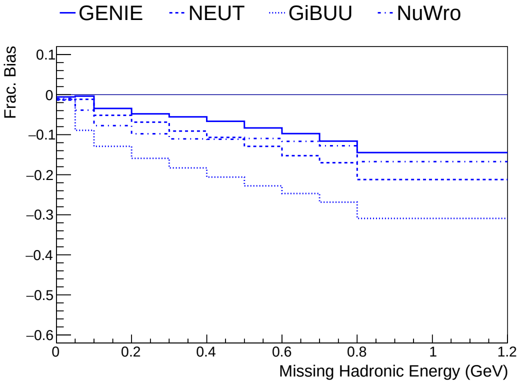


(b) $W^2$ method.

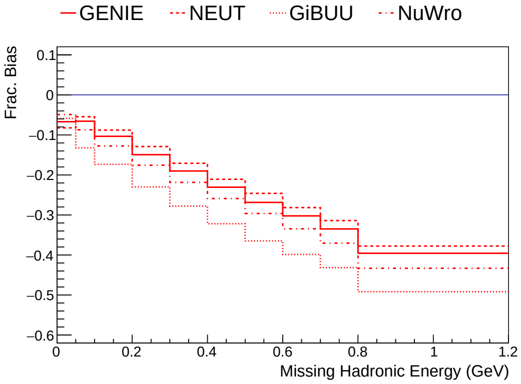


(c) MicroBooNE-like.

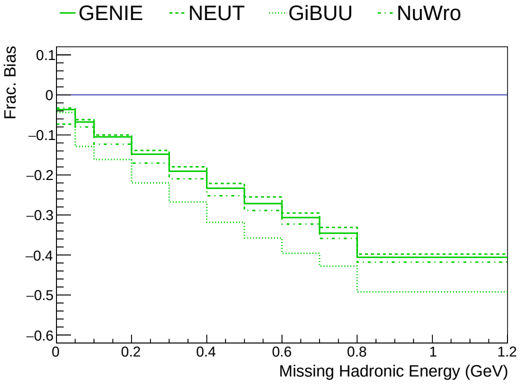


(d) SF method.

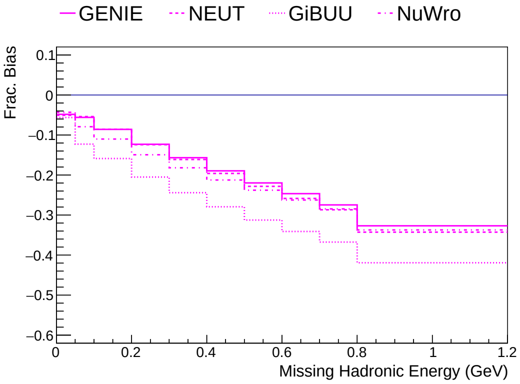


(e) Calorimetric method.

Figure 10: Bias in neutrino energy calculated as a function of missing hadronic energy, comparing the predictions from the different event generators for each estimator.

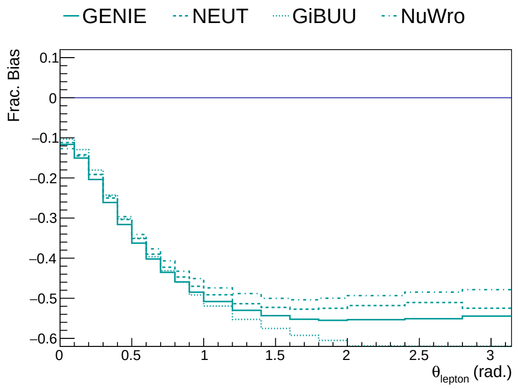


(a) Muon kinematics.

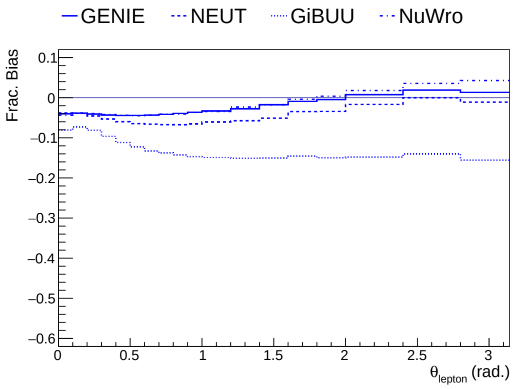


(b) $W^2$ method.

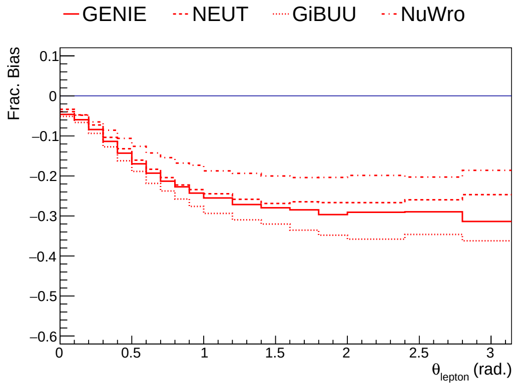


(c) MicroBooNE-like.

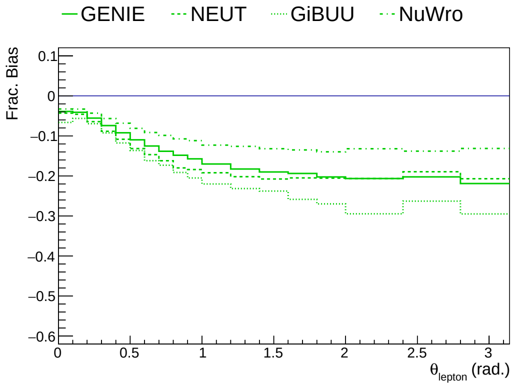


(d) SF method.

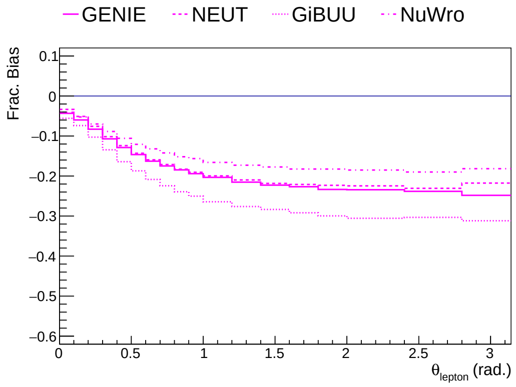


(e) Calorimetric method.

Figure 11: Bias in neutrino energy calculated as a function of lepton scattering angle, comparing the predictions from the different event generators for each estimator.

## 4 Event Distributions for Exclusions

Figs 12 and 13 contain the event distributions, all normalized to the same exposure, used to calculate the relative exclusion strengths discussed in Section VII of the article. These distributions are calculated using the DUNE flux [1] assuming oscillations at the baseline of the DUNE far detector.

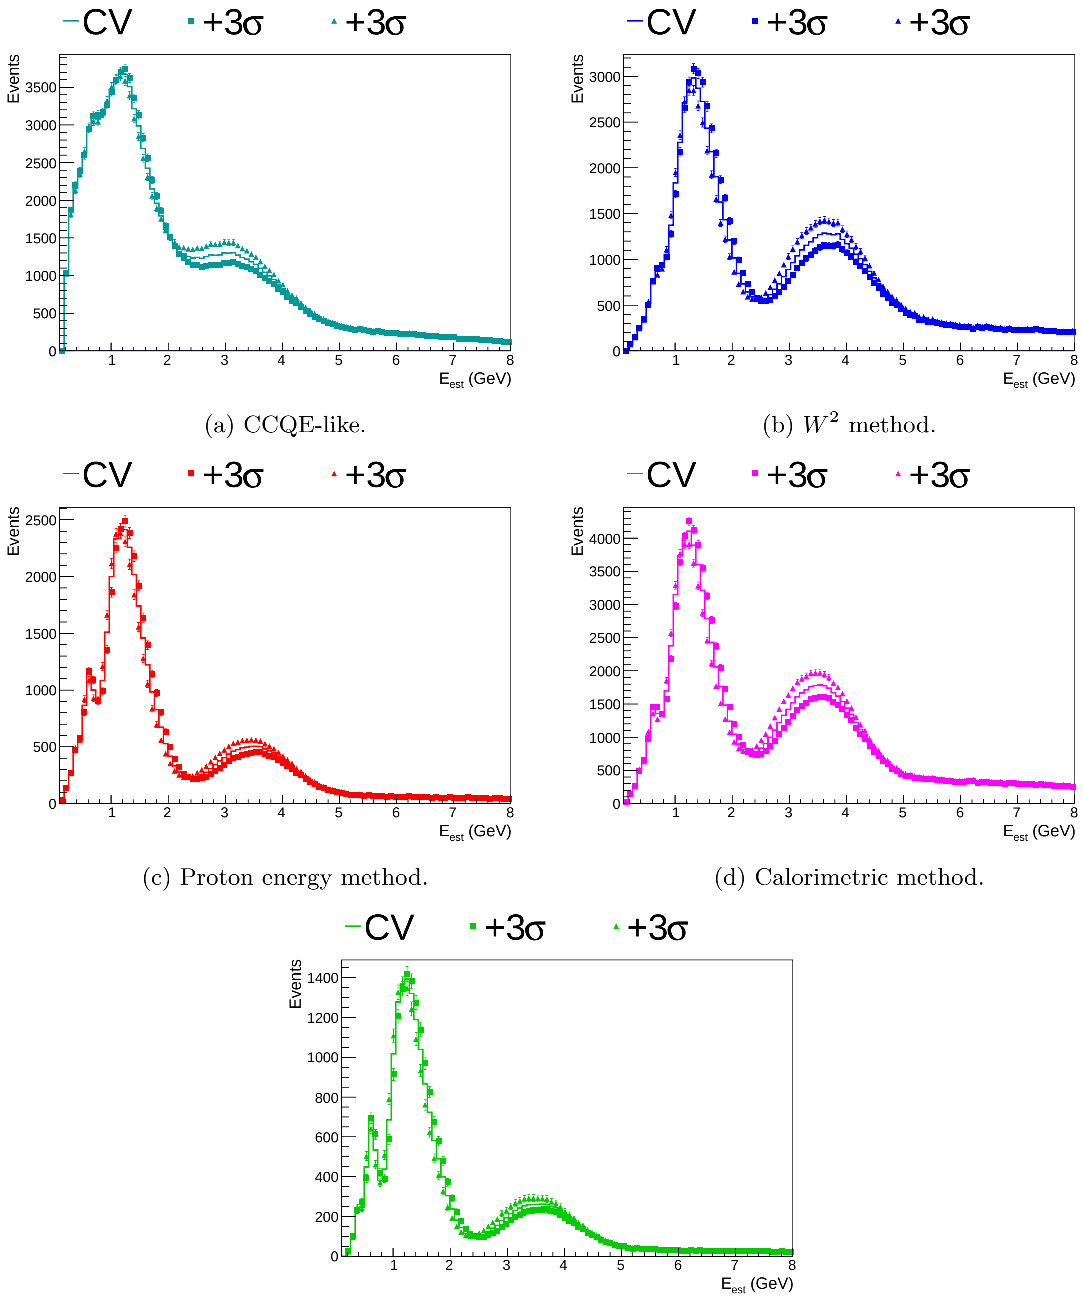


(a) CCQE-like.

(b) $W^2$ method.

(c) Proton energy method.

(d) Calorimetric method.

(e) Sobczyk-Furmanski.

Figure 12: Estimated energy distributions of events produced simulated $\nu_\mu$ interactions on argon using the DUNE flux, simulating $\nu_\mu$ disappearance at the baseline of the DUNE far detector.

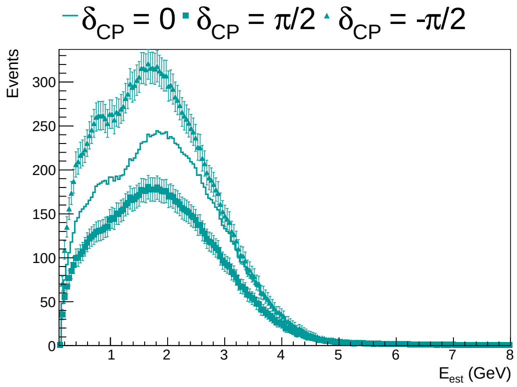


(a) CCQE-like.

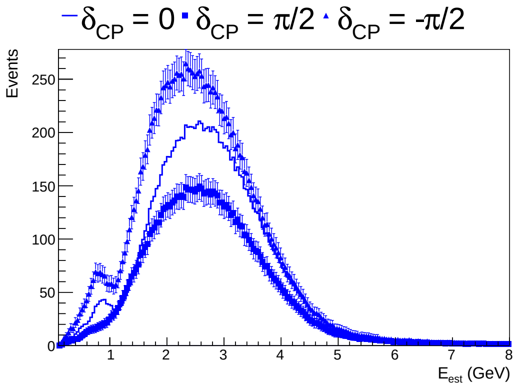


(b) $W^2$ method.

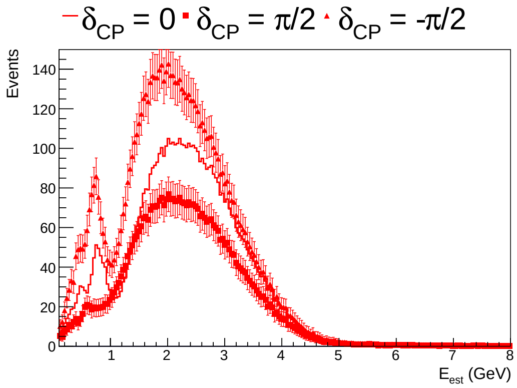


(c) Proton energy method.

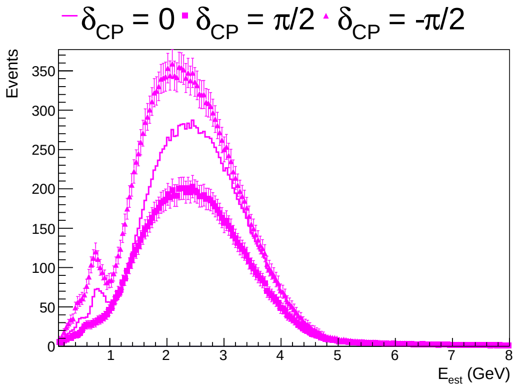


(d) Calorimetric method.

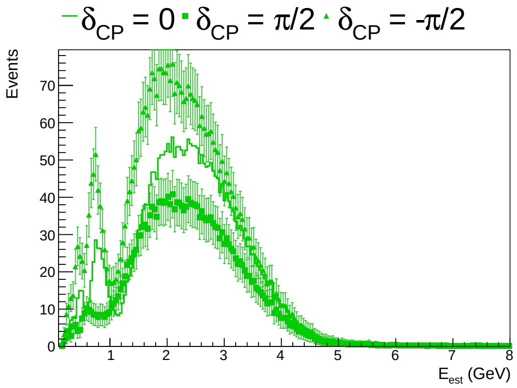


(e) Sobczyk-Furmanski.

Figure 13: Estimated energy distributions of events produced simulated $\nu_e$ interactions on argon using the DUNE flux, simulating $\nu_e$ appearance at the baseline of the DUNE far detector.

# References

[1] R. Acciarri *et al.* (DUNE), Long-Baseline Neutrino Facility (LBNF) and Deep Underground Neutrino Experiment (DUNE): Conceptual Design Report, Volume 2: The Physics Program for DUNE at LBNF (2015), arXiv:1512.06148 [physics.ins-det].

[2] A. P. Furmanski and J. T. Sobczyk, Neutrino energy reconstruction from one muon and one proton events, Phys. Rev. C **95**, no.6, 065501 (2017), arXiv:1609.03530 [hep-ex].
